# Supplementary material for: GENOT: Entropic (Gromov) Wasserstein Flow Matching with Applications to Single-Cell Genomics
Source: arXiv:2310.09254 source file (2024-11-07)
Supplement: Supplementary file 1 [file 6_appendix.tex]

\section{Appendix}
\subsection{Code submission}
We provide an anonymised version of the FlatVI code repository via \href{https://figshare.com/s/98de760e3aac23dbd399}{FigShare}.

\subsection{Derivation of the Fisher Information Metric for the Negative Binomial distribution}\label{app: derivation_fisher}
We first show that the Fisher Information of a univariate Negative Binomial (NB) distribution parameterised by mean $\mu$ and inverse dispersion $\theta$ with respect to $\mu$ is 
\begin{equation}
    \mathrm{M}(\mu) = \frac{\theta}{\mu(\mu+\theta)} \: .
\end{equation}
We then move on with the derivation of the pullback metric in \cref{prop:fisher_negative_binomial}.

\paragraph{Fisher Information of the NB distribution} The univariate NB probability distribution parameterised by mean $\mu$ and inverse dispersion $\theta$ is
\begin{equation}
p_{\textrm{NB}}(x \mid \mu, \theta)=\frac{\Gamma(\theta+x)}{x!\Gamma(\theta)}\Big(\frac{\theta}{\theta+\mu}\Big)^\theta\Big(\frac{\mu}{\theta+\mu}\Big)^x\: .
\end{equation}
The Fisher Information of the distribution can be computed with respect to $\mu$ as:
\begin{equation}\label{eq: fisher_info}
    \mathrm{M}(\mu) = -\mathbb{E}_{p(x \mid \mu, \theta)}\left[ \frac{\partial^2}{\partial \mu^2}\log p_\mathrm{NB}(x \mid \mu, \theta) \right] \; .
\end{equation} 
where 
\begin{equation}
    \log p_\mathrm{NB}(x \mid \mu, \theta) = C + \theta \left[\log(\theta)-\log(\theta+\mu)\right] + x\left[\log(\mu) - \log(\theta+\mu) \right] \; , \\
\end{equation}
with $C=\log(\Gamma(\theta+x))-\log(x!)-\log(\Gamma(\theta))$. Then, it can be shown that
\begin{equation}\label{eq: second_deriv_nb}
    \frac{\partial^2}{\partial \mu^2}\log p_\mathrm{NB}(x \mid \mu, \theta) = \frac{\theta+x}{(\theta+\mu)^2} - \frac{x}{\mu^2} \; .
\end{equation} 
Using the fact that the parameterisation involving the mean $\mu$ and inverse dispersion $\theta$ implies that
\begin{equation}
    \mathbb{E}_{p(x \mid \mu, \theta)}\left[x \right] = \mu \: ,
\end{equation}
we can expand \cref{eq: fisher_info} as follows
\begin{align}
    \mathrm{M}(\mu) &= -\mathbb{E}_{p(x \mid \mu, \theta)} \left[ \frac{\theta+x}{(\theta+\mu)^2} - \frac{x}{\mu^2}\right]\nonumber\\
    & =-\frac{1}{(\theta+\mu)^2}\mathbb{E}_{p(x \mid \mu, \theta)}\left[\theta + x \right] + \frac{1}{\mu^2}\mathbb{E}_{p(x \mid \mu, \theta)}\left[x\right]\\ 
    &= \frac{\theta}{\mu(\mu+\theta)} \: . \nonumber
\end{align}

\paragraph{Derivation of the Fisher Information Metric} We here consider the NB-VAE case, where the likelihood is parameterised by $\bm{\mu}_g=h_g(\mathbf{z})$ and $\bm{\theta}_g$ independently for each gene $g$.

When $h$ is a continuously differentiable function of $\mathbf{z}$, the pullback metric $\mathrm{M}_g(\mathbf{z})$ of the output $g$ w.r.t $\mathbf{z}$ by the reparameterisation property \citep{LehmCase98} is
\begin{align}
\mathrm{M}_g({\mathbf{z}}) & =\nabla_{\mathbf{z}}h_g(\mathbf{z})\mathrm{M}(h_g(\mathbf{z}))\nabla_{\mathbf{z}}h_g(\mathbf{z})^T \nonumber \\
 & =\frac{\bm{\theta}_g}{h_g(\mathbf{z})(h_g(\mathbf{z})+\bm{\theta}_g)}\nabla_{\mathbf{z}}h_g(\mathbf{z})\otimes\nabla_{\mathbf{z}}h_g(\mathbf{z})\: , 
\end{align}
where $\otimes$ is the outer product of vectors, and the gradients are column vectors.

By the chain rule, the joint Fisher Information of independent random variables equals the sum of the Fisher Information values of each variable \citep{zamirinf}. As all $\mathbf{x}_g$ are independent given $\mathbf{z}$ in the NB-VAE, the resulting Fisher Information Metric (FIM) is
\begin{align}\label{eq: fisher_rao_nb_supp}
\mathrm{M}(\mathbf{z}) & = \sum_g\mathrm{M}_g(\mathbf{z}) \nonumber\\
               & =\sum_g \frac{\bm{\theta}_g}{h_g(\mathbf{z})(h_g(\mathbf{z})+\bm{\theta}_g)}\nabla_\mathbf{z} h_g(\mathbf{z})\otimes\nabla_\mathbf{z} h_g(\mathbf{z}) \: .
\end{align}

% \subsection*{Extended background}

\subsection{The geometry of AEs}
We deal with the assumption that the observed data lies near a Riemannian manifold $\mathcal{M}_\sX$ embedded in the ambient space $\sX = \mathbb{R}^G$. The manifold $\mathcal{M}_{\sX}$ is defined as follows:

\begin{definition}
    A Riemannian manifold is a smooth manifold $\mathcal{M}_{\sX}$ endowed with a Riemannian metric $\mathrm{M}(\mathbf{x})$ for $\mathbf{x} \in \mathcal{M}_{\sX}$. $\mathrm{M}(\mathbf{x})$ changes smoothly and identifies an inner product on the tangent space $\mathcal{T}_\mathbf{x}\mathcal{M}_\mathcal{X}$ at a point $\mathbf{x} \in \mathcal{M}_{\mathcal{X}}$ as $\langle\mathbf{u}, \mathbf{v}\rangle_{\mathcal{M}_\mathcal{X}} = \mathbf{u}^\mathbf{T}\mathrm{M}(\mathbf{x})\mathbf{v}$, with $\mathbf{v}, \mathbf{u} \in \mathcal{T}_\mathbf{x}\mathcal{M}_\mathcal{X}$.
\end{definition}

For an embedded manifold $\mathcal{M_\mathcal{X}}$ with intrinsic dimension $d$, we can assume the existence of an invertible global chart map $\phi: \mathcal{M}_{\sX} \to \mathbb{R}^d$ mapping the manifold $\mathcal{M}_{\sX}$ to its intrinsic coordinates. A vector $\mathbf{v}_\mathbf{x}\in\mathcal{T}_\mathbf{x}\mathcal{M}_{\sX}$ on the tangent space of $\mathcal{M}_{\sX}$ can be expressed as a pushforward $\mathbf{v}_\mathbf{x}=\mathbb{J}_{\phi^{-1}}(\mathbf{z})\mathbf{v}_{\mathbf{z}}$ of a tangent vector $\mathbf{v}_\mathbf{z} \in \mathbb{R}^d$ at $\mathbf{z}=\phi(\mathbf{x})$, where $\mathbb{J}$ indicates the Jacobian. Therefore, $\mathbb{J}_{\phi^{-1}}$ maps vectors $\mathbf{v} \in \mathbb{R}^d$ into the tangent space of the embedded manifold $\mathcal{M}_\mathcal{X}$. Following \citet{geometrically_enriched}, the ambient metric $\mathrm{M}(\mathbf{x})$ can be related to the metric $\mathrm{M}(\mathbf{z})$ defined in terms of intrinsic coordinates via:
\begin{equation}\label{eq: pullback_coord}
    \mathrm{M}(\mathbf{z})=\mathbb{J}_{\phi^{-1}}(\mathbf{z})^T\mathrm{M}(\phi^{-1}(\mathbf{z}))\mathbb{J}_{\phi^{-1}}(\mathbf{z})\: .
\end{equation}
In other words, we can use the metric $\mathrm{M}(\mathbf{z})$ to compute quantities on the manifold, such as geodesic paths. However, for an embedded manifold $\mathcal{M}_{\sX}$, the chart map $\phi$ is usually not known. A workaround is to define the geometry of $\mathcal{M}_{\sX}$ on another Riemannian manifold $\mathcal{M}_\mathcal{Z}$ with a trivial chart map $\phi(\mathbf{z})=\mathbf{z}$ for $\mathbf{z}\in\mathcal{M}_\mathcal{Z}$, which can be mapped to $\mathcal{M}_\mathcal{X}$ via a smooth immersion $h$. In the next section, we elaborate on the connection between manifold learning and autoencoders following \citet{geometrically_enriched, arvanitidis2022pulling}. 

\subsubsection{Deterministic AEs}\label{app: geometry_autoencoders}
We assume the decoder $h: \mathcal{Z} = \mathbb{R}^d \rightarrow \mathcal{X} = \mathbb{R}^G$ of a deterministic autoencoder is an immersion of the latent space into a Riemannian manifold $\mathcal{M}_{\sX}$ embedded in $\sX$ and with metric $\mathrm{M}$. This is valid if one also assumes that $d$ is the intrinsic dimension of $\mathcal{M}_\sX$. As explained before, the Jacobian of the decoder maps tangent vectors $\mathbf{v}_\mathbf{z}\in\mathcal{T}_{\mathbf{z}}\mathcal{M}_\mathcal{Z}$ to tangent vectors $\mathbf{v}_{\mathbf{x}=h(\mathbf{z})}\in\mathcal{T}_\mathbf{x}\mathcal{M}_\mathcal{X}$. The decoder induces a metric into the latent space following \cref{eq: pullback_coord} as
\begin{equation}\label{eq: pullback_supp}
    \mathrm{M}(\mathbf{z})=\mathbb{J}_h(\mathbf{z})^T \mathrm{M}(h(\mathbf{z}))\mathbb{J}_h(\mathbf{z})\: ,
\end{equation}
called \textit{pullback metric}. The pullback metric defines the geometry of the latent manifold $\mathcal{M}_\mathcal{Z}$ in relation to that of the manifold $\mathcal{M}_\mathcal{X}$. The metric tensor $\mathrm{M}(\mathbf{z})$ regulates the inner product of vectors $\mathbf{u}$ and $\mathbf{v}$ on the tangent space $\mathcal{T}_\mathbf{z}\mathcal{M}_\mathcal{Z}$:
\begin{equation}
    \langle \mathbf{u}, \mathbf{v}\rangle_{\mathcal{M}_\mathcal{Z}} = \mathbf{u}^T\mathrm{M}(\mathbf{z})\mathbf{v}\: .
\end{equation}
To enhance latent representation learning, distances in the latent space \(\mathcal{Z}\) can be optimised according to quantities of interest in the observation space \(\mathcal{X}\), following the geometry of $\mathcal{M}_\sX$. For instance, we can define the length of a curve \(\gamma: [0, 1] \rightarrow \mathcal{Z}\) in the latent space by measuring its length on the manifold $\mathcal{M}_\sX$:
\begin{align}\label{eq: curve_len}
L(\gamma)   & =  \int_{0}^{1} \left\|{\dot{h}}(\gamma(t))\right\| \textrm{d}t \nonumber\\
            & = \int_{0}^{1} \sqrt{\dot{\gamma}(t)^T\mathrm{M}(\gamma(t))\dot{\gamma}(t)}\textrm{d}t \: ,
\end{align}

where the equality is derived by applying the chain rule of differentiation. 

\subsubsection{Pulling back the information geometry}\label{app: pullback_info}

In machine learning, exploring latent spaces is crucial, especially in generative models like VAEs. One challenge is defining meaningful distances in the latent space $\mathcal{Z}$, which often depends on the properties of stochastic decoders and their alignment with the observation space $\mathcal{X}$. Injecting the geometry of the decoded space of a VAE into the latent space requires a different theoretical framework, where the data is assumed to lie near a statistical manifold.

VAEs can model different kinds of data types by using the decoder function as a non-linear likelihood parameter estimation model. We consider the decoder's output space as a parameter space $\mathcal{H}$ for a probability density function. Depending on the data type, we express a likelihood function $p(\mathbf{x} \mid \bm{\theta})$ with parameters $\bm{\theta} \in \mathcal{H}$, reformulated as $p(\mathbf{x} \mid \mathbf{z})$ through a mapping $h: \mathcal{Z} \rightarrow \mathcal{H}$. We aim to define a natural distance measure in $\mathcal{Z}$ for infinitesimally close points $\mathbf{z}_1$ and $\mathbf{z}_2 = \mathbf{z}_1 + \delta \mathbf{z}$ when seen from $\mathcal{H}$. \citet{arvanitidis2022pulling} justify that such a distance corresponds to the Kullback-Leibler (KL) divergence:
\begin{equation}
   \text{dist}^2(\mathbf{z}_1, \mathbf{z}_2) = \text{KL}(p(\mathbf{x} \mid \mathbf{z}_1), p(\mathbf{x} \mid \mathbf{z}_2)) \: .
\end{equation}
To define the geometry of the statistical manifold, one can resort to information geometry, which studies probabilistic densities represented by parameters $\bm{\theta} \in \mathcal{H}$. In this framework, $\mathcal{H}$ becomes a statistical manifold equipped with a FIM:
\begin{equation}\label{eq: fim}
    \mathrm{M}(\bm{\theta}) = \int_\mathcal{X} [\nabla_{\bm{\theta}} \log p(\mathbf{x} \mid \bm{\theta})] [\nabla_{\bm{\theta}} \log p(\mathbf{x} \mid {\bm{\theta}})]^T p(\mathbf{x} \mid {\bm{\theta}}) \, \textrm{d}\mathbf{x} \: .
\end{equation}

The FIM locally approximates the KL divergence. For a univariate density $p$, parameterised by $\theta$, it is known that
\begin{equation}
   \text{KL}(p(x \mid \theta), p(x \mid \theta + \delta\theta)) \approx \frac{1}{2} \delta\theta^\top \mathrm{M}(\theta) \delta\theta + o(\delta\theta^2) \: .
\end{equation}
In the VAE setting, we view the decoder not as a mapping to the observation space $\mathcal{X}$ but as a transformation to the parameter space $\mathcal{H}$. This perspective allows us to naturally incorporate the FIM into the latent space $\mathcal{Z}$. Consequently, the VAE can be seen as spanning a manifold $h(\mathcal{Z})$ in $\mathcal{H}$, with $\mathcal{M}_\mathcal{Z}$ inheriting the metric in \cref{eq: fim} via the Riemannian pullback. Based on this, we define a statistical manifold.

\begin{definition}
    A statistical manifold is represented by a parameter space $\mathcal{H}$ of a distribution $p(\mathbf{x} \mid \bm{\theta})$ and is endowed with the FIM as the Riemannian metric. 
\end{definition}

The Riemannian pullback metric is derived as in \cref{eq: pullback_supp}. Having defined the Riemannian pullback metric for VAEs with arbitrary likelihoods, one can extend the measurement of curve lengths in $\mathcal{Z}$ when mapped to $\mathcal{H}$ through $h$ as displayed by \cref{eq: curve_len}. This approach allows flexibility in the choice of the decoder, as long as the FIM of the chosen distribution type is tractable.

\subsection{Baseline description}
Here, we describe the Geodesic Autoencoder (GAE) from \citet{mioflow}. For more details on the theoretical framework, we refer to the original publication. The GAE works by matching Euclidean distances between latent codes with the \textit{diffusion geodesic distance}, which is an approximation of the diffusion ground distance in the observation space. 

Briefly, the authors compute a graph with affinity matrix based on distances between observations $i$ and $j$ using a Gaussian kernel as:
\begin{equation}
    (\mathbf{K_\epsilon})_{ij}=k_\epsilon(\mathbf{x}_i, \mathbf{x}_j)\: ,
\end{equation}
with scale parameter $\epsilon$, where $\mathbf{x}_i, \mathbf{x}_j \in \mathcal{X}$ and $\mathcal{X}$ is the observation space. The affinity is then density-normalised by $\mathbf{M}_\epsilon=\mathbf{Q}^{-1}\mathbf{K}_\epsilon\mathbf{Q}^{-1}$, where $\mathbf{Q}$ is a diagonal matrix such that $\mathbf{Q}_{ii}=\sum_j(\mathbf{K_\epsilon
})_{ij}$. To compute the diffusion geodesic distance, the authors additionally calculate the diffusion matrix $\mathbf{P}_\epsilon=\mathbf{D}^{-1}\mathbf{M}_\epsilon$, with $\mathbf{D}_{ii}=\sum_{j=1}^n(\mathbf{M}_\epsilon)_{ij}$ and stationary distribution $\bm{\pi}_{i}=\mathbf{D}_{ii}/\sum_j\mathbf{D}_{jj}$. The diffusion geodesic distance between observations $\mathbf{x}_i$ and $\mathbf{x}_j$ is
\begin{equation}\label{eq: diffusion_geodesic_distance}
    G_\alpha(\mathbf{x}_i, \mathbf{x}_j) = \sum_{k=0}^{K}2^{-(K-k)\alpha}\lVert (\mathbf{P}_\epsilon)_{i:}^{2^{k}} - (\mathbf{P}_\epsilon)_{j:}^{2^{k}} \rVert_1 + 2^{-(K+1)/2}\lVert \bm{\pi}_i - \bm{\pi}_j\rVert_1 \: ,
\end{equation}
with $\alpha \in(0, 1/2)$. The running value of $k$ in \cref{eq: diffusion_geodesic_distance} defines the scales at which similarity between the random walks starting at $\mathbf{x}_i$ and $\mathbf{x}_j$ are computed.

Given the diffusion geodesic distance $G_\alpha$ defined in \cref{eq: diffusion_geodesic_distance}, the GAE model is trained such that the pairwise Euclidean distances between latent codes approximate the diffusion geodesic distances in the observation space $\mathcal{X}$, in a batch of size $B$. Given an encoder $f: \mathbb{R}^G \to \mathbb{R}^d$, the reconstruction loss is optimised alongside a geodesic loss
\begin{equation}
    \mathcal{L}_{\textrm{geodesic}} = \frac{2}{B}\sum_{i=1}^{N}\sum_{j>i}(\lVert f(\mathbf{x}_i) - f(\mathbf{x}_j) \rVert_2 - G_\alpha(\mathbf{x}_i, \mathbf{x}_j))^2\: .
\end{equation}

\subsection{Additional comparison between FlatVI and GAE}\label{sec: comparison_huguet}
Although related in scope, the proposed method significantly differs from the Geodesic Autoencoder (GAE) proposed by \citet{mioflow}. Firstly, GAE is a deterministic autoencoder optimised for reconstruction based on a Mean Squared Error (MSE) loss. As such, the model is not tailored to simulate gene counts. On the contrary, FlatVI optimises the decoder as an NB model, such that sampling from it produces discrete counts. This aspect has two advantages. By focusing on learning continuous parameters of a discrete likelihood, FlatVI explicitly models distributional properties of single-cell transcriptomics data, such as overdispersion, sparsity and discreteness. On the contrary, a fully connected Gaussian decoder produces dense and continuous cells, failing to preserve the characteristics of the data. Moreover, the GAE’s regularisation relies on the construction of a k-nearest-neighbourhood to approximate the geodesic distance between data points. This method requires the computation of pairwise Euclidean distances in the observation space. As suggested previously, gene expression is highly dimensional and, therefore, deceiving due to the Curse of Dimensionality. On the contrary, leveraging only the Jacobian and the output of the decoder to enforce latent space Euclideanicity, FlatVI is more suitable for larger datasets and eludes computing distances in high dimensions.

\subsection{Model setup}\label{sec:experimental_setup}

\begin{table}[]
\centering
\caption{Hyperparameter sweeps for training FlatVI. The hidden dimension column excludes the latent space layer, which is set to 10 unless specified otherwise. In bold, is the selected value used to present the results in the main.}
\begin{tabular}{@{}c|c|c|l@{}}
\toprule
                              & batch size   & hidden dims                                     & \multicolumn{1}{c}{$\lambda$} \\ \midrule
\multicolumn{1}{c|}{EB}       & \textbf{32}, 256, 512 & [1024, 512, 256], [512, 256], \textbf{[256]} & 0.001, 0.01, 0.1, \textbf{1}, 10       \\
\multicolumn{1}{c|}{Pancreas} & \textbf{32}, 256, 512 & [1024, 512, 256], [512, 256], \textbf{[256]} & 0.001, 0.01, 0.1, \textbf{1}, 10       \\
\multicolumn{1}{c|}{CMV}      & \textbf{32}, 256, 512 & [1024, 512, 256], [512, 256], \textbf{[256]} & 0.001, 0.01, 0.1,\textbf{ 1}, 10       \\
\multicolumn{1}{c|}{MEF}      & \textbf{32}, 256, 512 & [1024, 512, 256], [512, 256], \textbf{[256]} & 0.001, 0.01, \textbf{0.1}, 1, 10       \\ \bottomrule
\end{tabular}\label{tab: sweeps}
\end{table}

\paragraph{Experimental details for Autoencoder models} The Geodesic AE, NB-VAE and FlatVI models are trained via shallow 2-layer neural networks with hidden dimensions \texttt{[256, 10]}. Between consecutive layers, we include batch normalisation, as we found that it improves the reconstruction loss. Non-linearities are introduced by the \texttt{ELU} activation function. Models are trained for 1000 epochs monitoring the VAE loss for early stopping with a 20-epoch patience. The learning rate is set by default to \texttt{1e-3}. Additionally, we increase the KL divergence from 0 to 1 linearly across epochs in VAE models. The NB-VAE and FlatVI models are trained with a batch size of 32. For the geodesic AE model, we employed a batch size of 256 after sweeping all values in $\{64, 100, 256\}$. Importantly, the geodesic autoencoder was trained to reconstruct $\log$-normalised counts as opposed to the NB-VAE and FlatVI, since it does not assume a NB decoder. Finally, for training stability, all encoders are fed with $\log(1+\mathbf{x})$ given an input $\mathbf{x}$. The list of hyperparameter sweeps for FlatVI together with the selected values based on the validation loss is provided in \cref{tab: sweeps}.

\paragraph{Experimental details for OT-CFM} For OT-CFM we use a 3-layer MLP with 64 hidden units per layer, a \texttt{SELU} activation function and a learning rate of \texttt{1e-3}. The velocity network is fed with a latent state concatenated with a scalar representing the time used for interpolation. Following suggestions from the OT-CFM repository \footnote{\url{https://github.com/atong01/conditional-flow-matching}}, in each epoch we collect batches of cells from all time points to compute the objective for backpropagation. The variance hyperparameter $\sigma$ is set to 0.1 by default.

\paragraph{The choice of the hyperparameter $\lambda$} The hyperparameter $\lambda$ is crucial to control the degree of latent space flatness achieved by FlatVI. As denoted by Table~\ref{tab:tradeoff_lik_flatness}, a higher value of $\lambda$ corresponds to a more uniform (lower VoR) and flatter (lower MF) latent geometry at the price of a gradual decrease of the reconstruction quality. It is therefore important to choose a value of such a hyperparameter to ensure that flatness is enforced and reconstruction is good enough to predict realistic gene trajectories. In our experiments, we tested FlatVI followed by OT-CFM for different values of $\lambda$. Specifically, we increase the value of $\lambda$ as far as it produces an improved latent reconstruction by OT-CFM. For most datasets, increasing $\lambda$ from 0.1 to 1 produces performance increases in trajectory reconstruction, whereas moving from 1 to 10 does not and it is therefore not worth the likelihood decrease. For the more complex MEF dataset, moving from 0.1 to 1 did not improve OT-CFM-based trajectory reconstruction, so we decided to set $\lambda$ to 0.1.

\subsection{Evaluation metrics}

\subsubsection{Metric description}\label{app: metric_description}
\paragraph{Magnification factor} The magnification factor \citep{607494} is calculated as:
\begin{equation}
\textrm{MF}(\mathbf{z}) = \sqrt{\det \mathrm{M}(\mathbf{z})}\: .
\end{equation}
Here, $\mathrm{M}(\mathbf{z})$ represents the Riemannian metric tensor. Proximity to 1 reflects the similarity of the metric to the identity matrix.

\paragraph{Variance of the Riemannian metric}

In assessing the Riemannian metric, we introduce a key evaluation called the Variance of the Riemannian Metric (VoR) \citep{Pennec2006}. VoR is defined as the mean square distance between the Riemannian metric $\mathrm{M}(\mathbf{z})$ and its mean $\bar{\mathrm{M}} = \mathbb{E}_{\mathbf{z}\sim p_\mathbf{z}}[\mathrm{M}(\mathbf{z})]$. As suggested in \citet{lee2022regularized}, we compute the VoR employing an affine-invariant Riemannian distance metric $d$, expressed as:
\begin{equation}\label{eq: vor}
d^2(A, B) = \sum_{i=1}^{m} \left(\log \lambda_i(B^{-1}A)\right)^2\: ,
\end{equation}
where $\lambda_i(B^{-1}A)$ indicates the $i^{th}$ eigenvalue of the matrix $B^{-1}A$. VoR provides insights into how much the Riemannian metric varies spatially across different $\mathbf{z}$ values. When VoR is close to zero, it indicates that the metric remains constant throughout the support of $P_\mathbf{z}$. This evaluation procedure focuses solely on the spatial variability of the Riemannian metric and is an essential aspect of assessing the learned manifolds. Note that the expected value in \cref{eq: vor} is estimated using batches of latent observations with size 256.

\paragraph{Density}\citep{naeem2020reliable} Let $\mathbf{Y}$ and $\mathbf{X}$ be sets of generated and real data points with $M$ and $N$ observations, respectively. The neighbourhood sphere ${B(\mathbf{x}_i, \textrm{NND}_k(\mathbf{x}_i))}$ is the spherical region around a real datapoint $\mathbf{x}_i$ with, as radius, the distance between $\mathbf{x}_i$ and the furthest of its k-nearest neighbours. For a generated sample $\mathbf{y}_i$, Density evaluates the number of real neighbourhood spheres that encompass $\mathbf{y}_j$. Mathematically, the metric is defined as:
\begin{equation}
\text{Density}(\mathbf{X}, \mathbf{Y}) = \frac{1}{kM} \sum_{j=1}^{M} \sum_{i=1}^{N} \mathbbm{1}_{\mathbf{y}_j \in B(\mathbf{x}_i, \mathrm{NND}_k(\mathbf{x}_i))}\: .
\end{equation}
 The Density metric rewards generated samples situated in regions where real samples are densely clustered. Importantly, Density can be higher than 1.

\paragraph{Coverage}\citep{naeem2020reliable} Similar to Density, Coverage builds a k-nearest-neighbourhood around the real samples as the sphere ${B(\mathbf{x}_i, \textrm{NND}_k(\mathbf{x}_i))}$. Given real and generated samples $\mathbf{X}$ and $\mathbf{Y}$ with $N$ and $M$ observations, Coverage is defined as:
\begin{equation}
    \text{Coverage}(\mathbf{X}, \mathbf{Y}) = \frac{1}{N} \sum_{i=1}^{N} \left(\mathbbm{1}_{\exists j \text{ s.t.} \mathbf{y}_j \in B(\mathbf{x}_i, \textrm{NND}_k(\mathbf{x}_i))}\right)\: .
\end{equation}
Thus, Coverage measures the fraction of real samples whose neighbourhoods contain at least one generated sample. The score is bounded between 0 and 1.

\paragraph{Velocity Consistency}\citep{Gayoso2023} This metric quantifies the average Pearson correlation between the velocity $v(\mathbf{x}_j)$ of a reference cell $\mathbf{x}_j$ and the velocities of its neighbouring cells within the k-nearest-neighbour graph. It is mathematically expressed as:
\begin{equation}
    c_j = \frac{1}{k} \sum_{\mathbf{x} \in \mathcal{N}_k(\mathbf{x}_j)} \text{corr}(v(\mathbf{x}_j), v(\mathbf{x}))\: .
\end{equation}
Here $c_j$ represents the Velocity Consistency, $k$ denotes the number of nearest neighbours considered in the k-nearest-neighbour graph, $\mathbf{x}_j$ is the reference cell, $\mathcal{N}_k(\mathbf{x}_j)$ represents the set of neighbouring cells. The value $\text{corr}(v(\mathbf{x}_j), v(\mathbf{x}))$ is the Pearson correlation between the velocity of the reference cell $v(\mathbf{x}_j)$ and the velocity of each neighbouring cell $v(\mathbf{x})$. Higher values of $c_j$ indicate greater local consistency in velocity across the cell manifold. 

\subsubsection{Metric computation}\label{app: metric_comp}
\textbf{Trajectory reconstruction experiments} In Table~\ref{tab:leaveout_performance}, we explore the performance of OT on different embeddings based on the reconstruction of held-out time points. For most datasets, we evaluate the leaveout performance on all intermediate time points. The only exception is the MEF reprogramming dataset \citep{Schiebinger2019}, where we conduct our evaluation holding out time points 2, 5, 10, 15, 20, 25 and 30 to limit the computational burden of the experiment. After training OT-CFM excluding the hold-out time point $t$, we collect the latent representations of cells at $t-1$ and simulate their trajectory until time $t$, where we compare the generated cells with the ground truth via distribution matching metrics. Density and Coverage in the gene expression space are used to evaluate the mixing between the real and generated cells. Their values are computed in the PCA space of 50 dimensions of the $\log$-transformed real and generated gene counts, considering 10 neighbours. Finally, for the latent reconstruction quantification, generated latent cell distributions at time $t$ are standardised with the mean and standard deviation of the latent codes of real cells at time $t$ to make the results comparable across embedding models. Results in \cref{tab:leaveout_performance} are averaged across three seeds.

\textbf{Fate mapping with CellRank} Following the setting proposed by \citet{eyring2022modeling}, we compute the latent velocity field with OT-CFM and input the velocities to CellRank \citep{Lange2022, Weiler2023}. Using the function \texttt{g.compute\_macrostates(n\_states, cluster\_key)} of the GPPC estimator for macrostate identification \citep{Reuter2018}, we look for 10 to 20 macrostates. If OT-CFM cannot find one of the 6 terminal states within 20 macrostates for a certain representation, we mark the terminal state as missed (see Figure~\ref{fig:cellrank_experiment}). Terminal states are computed with the function \texttt{compute\_terminal\_states(method, n\_states)}. Velocity consistency is estimated using the scVelo package \citep{Bergen2020} through the function \texttt{scv.tl.velocity\_confidence(adata\_latent\_flat)}. The value is then averaged across cells.  

\textbf{Lineage driver analysis Figure~\ref{fig:rnaseq_simulation}b} We examine if lineage driver expression matches between real and predicted expression data. OT-based simulations are performed by pushing forward cells at time point $t_0$ using the learnt integration map. Pushed-forward cells are not annotated. We use label transfer to label cell clusters in the generated datasets based on the real data using the \texttt{sc.tl.ingest} Scanpy function \citep{Wolf2018}.

\subsection{Data}
\subsubsection{Data description}
\label{app:data}

\textbf{Embryoid Body (EB)} \cite{Moon2019} measured the expression of 18,203 differentiating human embryoid single cells across 5 time points. From an initial population of stem cells, approximately four lineages emerged, including Neural Crest, Mesoderm, Neuroectoderm and Endoderm cells. Here, we resort to a reduced feature space of 1241 highly variable genes. OT has been readily applied to the embryoid body datasets in multiple scenarios \citep{Tong2020TrajectoryNet, tong2023}, making it a solid benchmark for time-resolved single-cell trajectory inference. The data is split into 80\% training and 20\% test sets.

\textbf{Pancreatic Endocrinogeneris (Pancreas)} We consider 16,206 cells from \cite{BastidasPonce2019} measured across 2 time points corresponding to embryonic days 14.5 and 15.5. In the dataset, multipotent cells differentiate branching into endocrine and non-endocrine lineages until reaching 6 terminal states. Challenges concerning such dataset include bifurcation and unbalancedness of cell state distributions across time points \citep{eyring2022modeling}. The data is split into 80\% training and 20\% test sets.

\textbf{Infection Dataset (CVM)} We include the single-cell dataset from \cite{Hein2021} which profiles 12,919 fibroblasts infected by Cytomegalovirus across 7 time points. For trajectory inference, we subset the dataset to include only the human genome with the 2000 top highly variable genes. A challenge with this dataset is its reduced number of observations compared with its counterpart examples. The data is split into 90\% training and 10\% test sets.

\textbf{Reprogramming Dataset (MEF)}  We consider the dataset introduced in \citet{Schiebinger2019}, which studies the reprogramming of Mouse Embryonic Fibroblasts (MEF) into induced Pluripotent Stem Cells (iPSC). The dataset consists of 165,892 cells profiled across 39 time points and 7 cell states. For this dataset, we keep 1479 highly variable genes. Due to its number of cells, such a dataset is the most complicated to model among the considered. The data was split into 80\% training and 20\% test sets.

\subsubsection{Data preprocessing}
We use the Scanpy \citep{Wolf2018} package for single-cell data preprocessing. The general pipeline involves normalisation via \texttt{sc.pp.normalize\_total}, $\log$-transformation via \texttt{sc.pp.log1p} and highly-variable gene selection using \texttt{sc.pp.highly\_variable\_genes}. 50-dimensional embeddings are then computed via PCA through \texttt{sc.pp.pca}. We then use the PCA representation to compute the 30-nearest-neighbour graphs around single observations and use them for learning 2D UMAP embeddings of the data. For the latter steps, we employ the Scanpy functions \texttt{sc.pp.neighbours(adata)} and \texttt{sc.tl.umap(adata)}. For the CMV dataset \citep{Hein2021}, we exclude the viral genome and only keep human gene expression. Raw counts are preserved in \texttt{adata.layers["X\_counts"]} to train FlatVI.

\subsection{Details about computational resources}
Our model is implemented in Python 3.10, and for deep learning models, we used PyTorch 2.0. For the implementation of NeuralODE-based simulations, we use the torchdyn package. Our experiments ran on different GPU servers with varying specifications: GPU: 16x Tesla V100 GPUs (32GB RAM per card) / GPU: 2x Tesla V100 GPUs (16GB RAM per card) / GPU: 8x A100-SXM4 GPUs (40GB RAM per card)

\subsection{Algorithm}\label{sec: algorithms}
\begin{algorithm}[H]
   \caption{Train FlatVI}
   \label{alg:cap}
   \begin{algorithmic}
      \REQUIRE Data matrix $\mathbf{X}\in\mathbb{N}_0^{N \times G}$, batch size $B$, maximum iterations $n_{\mathrm{max}}$, encoder $f_\psi$, decoder $h_\phi$, flatness loss scale $\lambda$
      \ENSURE Trained encoder $f_\psi$, decoder $h_{\phi}$, and inverse dispersion parameter $\bm{\theta}$
      \STATE Randomly initialize gene-wise inverse dispersion $\bm{\theta}$
      \STATE Randomly initialize the identity matrix scale $\alpha$ as a trainable parameter
      \FOR {$i=1$ \textbf{to} $n_{\mathrm{max}}$}
         \STATE Sample batch $\mathbf{X}^b \gets \{\mathbf{x}_1,...,\mathbf{x}_B\}$ from $\textbf{X}$
         \STATE $\mathbf{l}^b \gets$ \texttt{compute\_size\_factor}$(\mathbf{X}^b)$
         \STATE $\mathbf{Z}^b \gets f_\psi(1+\log \mathbf{X}^b)$ 
         \STATE $\bm{\mu} \gets h_\phi(\mathbf{Z}^b, \mathbf{l}^b)$
         \STATE $\mathcal{L}_{\textrm{KL}} \gets$ \texttt{compute\_kl\_loss}$(\mathbf{Z}^b)$
         \STATE $\mathcal{L}_{\textrm{recon}} \gets$ \texttt{compute\_nb\_likelihood}$(\mathbf{X}^b, \bm{\mu}, \bm{\theta})$
         \STATE $\mathrm{M}(\mathbf{Z}^b) \gets$ \cref{eq: fisher_rao_nb_supp}
         \STATE $\mathcal{L}_{\textrm{flat}} \gets$ \texttt{MSE}$(\mathrm{M}(\mathbf{Z}^b), \alpha \mathbb{I}_d)$
         \STATE $\mathcal{L} = \mathcal{L}_{\textrm{recon}} + \mathcal{L}_{\textrm{KL}} + \lambda\mathcal{L}_{\textrm{flat}}$
         \STATE Update parameters via gradient descent
      \ENDFOR
   \end{algorithmic}
\end{algorithm}

\newpage
\begin{algorithm}[H]
   \caption{Train latent OT-CFM with FlatVI}
   \label{alg:cap}
   \begin{algorithmic}
      \REQUIRE Datasets $\{\mathbf{X}_t\}_{t=0}^T$, variance $\sigma$, batch size $B$, initial velocity function $v_\xi$, maximum iterations $n_{\max}$, trained encoder $f_\psi$
      \ENSURE Trained velocity function $v_\xi$
      \STATE $\{\mathbf{Z}_t\}_{t=0}^T \gets f_\psi (\{1+\log\mathbf{X}_t\}_{t=0}^T)$
      \STATE $\{\mathbf{l}_t\}_{t=0}^T \gets$ \texttt{compute\_size\_factor}$(\{\mathbf{X}_t\}_{t=0}^T)$
      \STATE $\{\mathbf{S}_t\}_{t=0}^T \gets$ \texttt{timewise\_concatenate}($\{\mathbf{Z}_t\}_{t=0}^T$, $\{\mathbf{l}_t\}_{t=0}^T$)
      \FOR {$i=1$ \textbf{to} $n_{\max}$}
         \STATE Initialize empty array of velocity predictions $\mathbf{V}$
         \STATE Initialize empty array of velocity ground truth $\mathbf{U}$
         \FOR {$t_{\mathrm{traj}}=0$ \textbf{to} $T-1$}
            \STATE Randomly sample batches with $B$ observations $\mathbf{S}^b_{t_{\mathrm{traj}}}$, $\mathbf{S}^b_{t_{\mathrm{traj}}+1}$
            \STATE $\pi \gets$ OT($\mathbf{S}^b_{t_{\mathrm{traj}}}$, $\mathbf{S}^b_{t_{\mathrm{traj}}+1}$)
            \STATE ($\mathbf{S}^b_{t_{\mathrm{traj}}}$, $\mathbf{S}^b_{t_{\mathrm{traj}}+1}$) $\sim \pi$
            \STATE $t\sim \mathcal{U}(0,1)$
            \STATE $\mathbf{S}^b \gets \mathcal{N}(t\mathbf{S}^b_{t_{\mathrm{traj}}}+(1-t)\mathbf{S}^b_{t_{\mathrm{traj}}+1}, \sigma^2\mathbb{I}_d)$
            \STATE Append $v_\xi(t+t_{\mathrm{traj}}, \mathbf{S}^b)$ to $\mathbf{V}$
            \STATE Append $(\mathbf{S}^b_{t_{\mathrm{traj}}+1}-\mathbf{S}^b_{t_{\mathrm{traj}}})$ to $\mathbf{U}$
         \ENDFOR
         \STATE $\mathcal{L}_{\mathrm{OT-CFM}} \gets \lVert \mathbf{V}-\mathbf{U}  \rVert^2$
         \STATE Update parameters via gradient descent
      \ENDFOR
   \end{algorithmic}
\end{algorithm}

\newpage
\subsection{Additional results}\label{sec: rna_velo}
We compared our whole pipeline involving the combination of FlatVI and OT-CFM with the scVelo \citep{Bergen2020} and veloVI \citep{Gayoso2023} models for RNA velocity analysis. \cref{fig: supp_4} and \cref{tab:terminal-consistency} show examples of how our approach favourably compares with velocity estimation methods, namely inferring a proper velocity field in Acinar cells and detecting all terminal states with high velocity consistency in the Pancreas dataset.

\begin{figure}[H]
\centering
\includegraphics[width=0.6\textwidth]{figures/supp_4.pdf}% Replace 'example-image' with the filename of your image
    \caption{Comparison between the vector field learnt on the Acinar branch of the Pancreas dataset by using OT-CFM in combination with FlatVI and standard RNA velocity algorithms.}\label{fig: supp_4}
\end{figure}

\begin{table}[H]
\centering
\caption{Number of terminal states computed by CellRank and velocity consistency using the representations and velocities learnt by FlatVI+OT-CFM and standard RNA velocity algorithms. }
\begin{tabular}{@{}c|c|c@{}}
\toprule
Method & Terminal states & Consistency \\ \midrule
FlatVI + OT-CFM & \textbf{6 }& \textbf{0.94} \\
veloVI & 5 & 0.92 \\
scVelo & 4 & 0.80 \\ \bottomrule
\end{tabular}\label{tab:terminal-consistency}
\end{table}

% \begin{figure}[H]
%     \centering
% \includegraphics[width=0.7\textwidth]{figures/supp_5.pdf} % Replace 'example-image' with the filename of your image
%     \caption{Comparison between trajectories generated by FlatVI+OT and the velocity model scTour in the EB datasets. }
% \end{figure}

% \begin{table}[H]
%     \centering
%     \caption{Wasserstein distance of marker expression between real and predicted values for different lineages considering FlatVI+OT-CFM and scTour.}
%     \begin{tabular}{@{}l|c|c@{}}
%         \toprule
%         Lineage & FlatVI+OT-CFM & scTour \\ \midrule
%         Neural crest & \textbf{0.04} & 0.07 \\
%         Neuronal & \textbf{0.02}& 0.03 \\
%         Cardiac & \textbf{0.07} & 0.27 \\
%         Endoderm & 0.05 & \textbf{0.03} \\ \bottomrule
%     \end{tabular}
%     \label{tab:marker-expression-distance}
% \end{table}
